# Supplementary material for: A Fully Problem-Dependent Regret Lower Bound for Finite-Horizon MDPs
Source: arXiv:2106.13013 source file (2021-06-24)
Supplement: Supplementary file 1 [file appendix.tex]

% !TEX root = main.tex 
\section{Problem-Dependent Lower Bound}

\subsection{Lower Bound Derivation (Proof of Theorem~\ref{th:main-lower-bound})}

\subsection{Analysis of the Lower Bound}

\subsection{The Impact of the Dynamics Constraint}

\subsection{The Full-Support Case}

\subsection{The Case of Known Dynamics: Reduction to Combinatorial Semi-bandits}

\section{Examples with Specific MDP Instances}

\subsection{Hard MDP from \citet{xu2021fine}}

\subsection{Dependence on the Minimum Gap}

\section{Policy-Gap Dependent Regret Bound for Optimistic Algorithms}

\section{Auxiliary Results}
